# Supplementary material for: A Self-adaptive Weighted Differential Evolution Approach for Large-scale Feature Selection
Source: arXiv:2110.14166 source file (2021-10-27)
Supplement: Supplementary file 1 [file Supplementary.tex]

\begin{document}
\title{Supplementary Materials to ``A Self-adaptive Weighted Differential Evolution Approach for Large-scale Feature Selection''}

\end{document}
